# Supplementary material for: SketchEmbedNet: Learning Novel Concepts by Imitating Drawings
Source: arXiv:2009.04806 source file (2021-06-22)
Supplement: Supplementary file 1 [file arch_comparisons.tex]

\section{Autoregressive drawing model comparisons}
\label{appendix:autoreg_draw_model_comp}
We summarize the key components of \modelembedding{} in comparison to other autoregressive drawing models in Table \ref{tab:sketch_arch_comparison}.
\begin{table*}[H]
    \centering
    \caption{Model comparisons between generative autoregressive models that produce pixel or vector sketch drawings.}
    \resizebox{0.98\textwidth}{!}{
    % model - dataset - # classes - encoder - decoder - loss 
    \begin{tabular}{@{}llllll@{}}
\toprule
\multicolumn{6}{c}{\textbf{Autoregressive sketching models}} \\ 
\midrule
\textbf{Model} & \textbf{Dataset} & \textbf{\# classes} & \textbf{Encoder} & \textbf{Decoder} & Loss function \\
\midrule
Handwriting Sequence \cite{gravesrnn} & IAM-OnDB \cite{iamondb} & 1 & RNN & Mixture Density RNN & $\mathcal{L}_\text{stroke}$ \\
DRAW \cite{draw} & SVHN\cite{svhn}, MNIST \cite{mnist} & 10 & RNN & RNN & $\mathcal{L}_\text{pixel} + \mathcal{L}_\text{KL}$ \\
Sketch-RNN \cite{ha2017sketchrnn} & Quickdraw \cite{jongejan2016quickdraw} & 1 & Bi-directional RNN & Mixture Density RNN & $\mathcal{L}_\text{pen} + \mathcal{L}_\text{stroke} + \mathcal{L}_\text{KL}$ \\
Sketch-pix2seq \cite{chen2017pix2seq} & Quickdraw \cite{jongejan2016quickdraw} & 3, 6 & simple CNN & Mixture Density RNN & $\mathcal{L}_\text{pen} + \mathcal{L}_\text{stroke}$ \\
AI-Sketcher \cite{aisketcher} & \makecell[l]{Quickdraw \cite{jongejan2016quickdraw}, \\ FaceX \cite{aisketcher}} & 5, 10, 15, 20 & \makecell[l]{Bi-directional RNN \\+ CNN Autoencoder} & Mixture Density RNN & $\mathcal{L}_\text{pen} + \mathcal{L}_\text{stroke} + \mathcal{L}_\text{KL}$ \\
deep\_p2s \cite{learn2sketchcycle} & \makecell[l]{Quickdraw \cite{jongejan2016quickdraw}, \\ ShoesV2 \cite{sketchshoe}, ChairV2} & 1 & Bi-directional RNN, CNN & CNN, Mixture Density RNN & \makecell[l]{$\mathcal{L}_\text{pen} + \mathcal{L}_\text{stroke} + \mathcal{L}_\text{l2}$ \\ $+ \mathcal{L}_\text{KL} + \mathcal{L}_\text{shortcut}$} \\
\midrule
\model{} \textit{(ours)} & Quickdraw \cite{jongejan2016quickdraw} & 300 & ResNet12 \cite{oreshkin2018tadam} & Mixture Density RNN & $\mathcal{L}_\text{pen} + \mathcal{L}_\text{stroke} + \mathcal{L}_\text{pixel}$ \\
\bottomrule
    \end{tabular}}
    \label{tab:sketch_arch_comparison}
\end{table*}
