# Supplementary material for: SketchEmbedNet: Learning Novel Concepts by Imitating Drawings
Source: arXiv:2009.04806 source file (2021-06-22)
Supplement: Supplementary file 2 [file baseline_embedding_properties.tex]

\section{Embedding properties of other baseline models}
\label{appendix:additional_embedding_baselines}
Here we substantiate the uniqueness of the properties observed in \modelembedding{}s by applying the same experiments to a $\beta$-VAE~\citep{betavae} as well a vanilla autoencoder trained on the same dataset. We also include results of a \model{} trained with a KL objective.

\subsection{$\beta$-VAE}
\begin{figure*}
    \centering
    \includegraphics[trim=2.3cm 1cm 2.3cm 1.35cm,clip,width=0.93\textwidth]{primaryfigs/appendixfigs/beta-VAE_figure_1.pdf}
    \caption{Section \ref{sec:compositionality} clustering results for $\beta$-VAE}
    \label{fig:betavae_cc_cluster}
\end{figure*}
\begin{figure*}
    \centering
    \includegraphics[trim=2.3cm 11.7cm 2.3cm 1.1cm,clip,width=0.93\textwidth]{primaryfigs/appendixfigs/beta-VAE_figure_2.pdf}
    \caption{Section \ref{sec:compositionality} conceptual composition results for $\beta$-VAE}
    \label{fig:betavae_cc_arithmetic}
\end{figure*}
The $\beta$-VAE~\citep{betavae} exhibits similar unsupervised clustering in comparison to the Conv-VAE and is generally incapable of distinguishing input images that have different shape compositions but the same overall silhouette (first two examples from the left). Differently it is better at distinguishing non-synthetic examples that contain multiple squares or circles (3rd figure). However, it utterly fails the latent variable regression task and does not exhibit any significant conceptual composition in latent space. 

\subsection{Autoencoder and \model-KL}
\begin{figure*}
    \centering
    \includegraphics[trim=0.5cm 4.3cm 0.5cm 2.5cm,clip,width=0.93\textwidth]{primaryfigs/appendixfigs/sketchEmbedNetKL_AE figures_1.pdf}
    \caption{Section \ref{sec:compositionality} clustering results for Autoencoder and \modelembedding{}-KL}
    \label{fig:autoencoder_draw_modelcc_cluster}
\end{figure*}
\begin{figure*}
    \centering
    \includegraphics[trim=0.5cm 11cm 0.5cm 2.4cm,clip,width=0.93\textwidth]{primaryfigs/appendixfigs/sketchEmbedNetKL_AE figures_2.pdf}
    \caption{Section \ref{sec:compositionality} conceptual composition results for Autoencoder and \modelembedding{}-KL}
    \label{fig:autoencoder_draw_modelcc_arithmetic}
\end{figure*}
We show that the performance of \modelembedding{} embeddings in our experiments in Section \ref{sec:compositionality} which focuses on organization in latent space is not correlated with the KL term. We present both a vanilla autoencoder without the KL objective and a \model{} trained with a KL objective. We observe a drop in overall generation quality in the Conceptual Composition decoding as is expected with an additional constraint but maintained performance in the other tasks. Meanwhile, the autoencoder does not demonstrate any marked improvements over the Conv-VAE in the main paper or any other baseline comparison.
