# Supplementary material for: SketchEmbedNet: Learning Novel Concepts by Imitating Drawings
Source: arXiv:2009.04806 source file (2021-06-22)
Supplement: Supplementary file 3 [file compositionality.tex]

\section{Additional compositionality modes}
\label{appendix:compositionality_modes}
We provide additional clustering methods t-SNE \citep{tsne} and PCA as well as 2 new experiments that explore the compositionality of our latent \modelembedding{}.

\paragraph{Additional clustering methods}
We include additional t-SNE and PCA results of the experiments in the main paper. These are presented in Figures \ref{fig:angle_dist}, \ref{fig:lin_dist}, \ref{fig:four} \ref{fig:inout}, \ref{fig:num_shapes}. t-SNE and UMAP are stochastic and do not always produce the same visualization while PCA is deterministic and prioritizes the most important dimensions. 

\begin{figure}[H]
    \centering
    \includegraphics[trim=0cm 2cm 6cm 0cm,clip,width=0.8\textwidth]{primaryfigs/appendixfigs/compositionality_figs_appendix/angle_legended.pdf}
    \caption{2D Embedding visualization of different spatial orientations of circles and squares}
    \label{fig:angle_dist}
\end{figure}
\begin{figure}[H]
    \centering
    \includegraphics[trim=0cm 2cm 6cm 0cm,clip,width=0.8\textwidth]{primaryfigs/appendixfigs/compositionality_figs_appendix/distance_legended.pdf}
    \caption{2D Embedding visualization of different linear distances between shapes}
    \label{fig:lin_dist}
\end{figure}
\begin{figure}[H]
    \centering
    \includegraphics[trim=0cm 2cm 6cm 0cm,clip,width=0.8\textwidth]{primaryfigs/appendixfigs/compositionality_figs_appendix/four_legended.pdf}
    \caption{Latent space visualization squares and circles arranged differently in a 2x2 array}
    \label{fig:four}
    \vspace*{-0.25in}
\end{figure}
\begin{figure}[H]
    \centering
    \includegraphics[trim=0cm 2cm 6cm 0cm,clip,width=0.8\textwidth]{primaryfigs/appendixfigs/compositionality_figs_appendix/inout_legended.pdf}
    \caption{Latent space visualization of composing circles and squares within one another or outside}
    \label{fig:inout}
    \vspace*{-0.25in}
\end{figure}
\begin{figure}[H]
    \centering
    \includegraphics[trim=0cm 2cm 6cm 0cm,clip,width=0.8\textwidth]{primaryfigs/appendixfigs/compositionality_figs_appendix/compositionality_legended.pdf}
    \caption{Latent space visualization of composing multiple circles and squares in real sketch drawings}
    \label{fig:num_shapes}
    \vspace*{-0.25in}
\end{figure}

\paragraph{Additional Experiments}
Here we provide different investigations into the compositionality of our learned embedding space that were not present in our main paper. These results presented in Figure \ref{fig:orientation} and \ref{fig:num_shapes_toy}. 

\begin{figure}[H]
    \centering
    \includegraphics[trim=0cm 2cm 6cm 0cm,clip,width=0.8\textwidth]{primaryfigs/appendixfigs/compositionality_figs_appendix/orientation_legended.pdf}
    \caption{2D Embedding visualization of different spatial orientations of circles and squares}
    \label{fig:orientation}
    \vspace*{-0.25in}
\end{figure}
In Figure \ref{fig:orientation} we place a square in the center of the example and place a circle above, below or to the sides of it. Once again we find that our \modelembedding{} embedding clusters better than the VAE approach.

\begin{figure}[H]
    \centering
    \includegraphics[trim=0cm 2cm 6cm 0cm,clip,width=0.8\textwidth]{primaryfigs/appendixfigs/compositionality_figs_appendix/count_toy_legended.pdf}
    \caption{Latent space visualization of composing multiple circles and squares in real sketch drawings}
    \label{fig:num_shapes_toy}
    \vspace*{-0.25in}
\end{figure}
New examples are generated where each class has a different numbers of circles. Both the VAE approach and our \modelembedding{} cluster well and neither appear to learn the count manifold.
