# Supplementary material for: SketchEmbedNet: Learning Novel Concepts by Imitating Drawings
Source: arXiv:2009.04806 source file (2021-06-22)
Supplement: Supplementary file 4 [file hypernetwork_activations.tex]

\section{HyperNetwork Activations}
\label{appendix:hypernetworks}
To further explore how our network understands drawings, we examine the relationships between the activations of the hypernetwork of our HyperLSTM \citep{ha2013hypernetworks}. 

The hypernetwork determines the weights of the LSTM that generates the RNN at each decoding timestep. These activations are 512-dimensional vectors. We collect the activations from many examples, cluster them in 512-dimensional space and visualize the strokes belonging to each cluster for each example. A full decoding is also rendered where each cluster within an example is assigned a color.

Figures~\ref{fig:snowman_hyper_activations_compose},~\ref{fig:allround_hyper_activations_compose},~\ref{fig:all_hyper_activations_compose} show class examples from different clustering runs where each cluster is assigned its own color. In Figures~\ref{fig:snowman_hyper_activations},~\ref{fig:allround_hyper_activations},~\ref{fig:all_hyper_activations} each row is a separate example. The input image is shown in the first column and ``noise'' strokes in the second and every subsequent column is a cluster. Some clusters are large with strokes coming from a whole number of example while others are fairly unique and only contain strokes from a single or few select examples. \MR{I suggest getting rid of Figure 11, 13 and 15 since they are very big and you probably want to condense the results in the final version}

\paragraph{Single class: snowman}
First we explore this clustering using only the snowman class from Quickdraw \citep{jongejan2016quickdraw}. We expect substantial reuse of a ``circle'' both within and over many examples. Clustering of the strokes is done with the DBSCAN \citep{dbscan} and parameter $\epsilon=3.9$. Results are in Figure \ref{fig:snowman_hyper_activations}.
\begin{figure*}[t]
    \vspace*{-0.1in}
    \centering
    \includegraphics[width=0.98\textwidth]{primaryfigs/compositionality_figs/hyper_activations/snowman/collage.png}
    \caption{Clustering of hypernetwork activations of over many generated sketches of snowmen. Left column is the full sketch, second are the ``noise'' strokes and every subsequent column is a unique cluster of stroke activations.}
    \label{fig:snowman_hyper_activations}
    \vspace*{-0.2in}
\end{figure*}
While cluster re-use is limited, cluster 0 often contains a large, fully enclosed circle. Many other clusters may contain circles or partial strokes with some reuse. Larger, fully composed and coloured sketches are presented in Figure \ref{fig:snowman_hyper_activations_compose}
\begin{figure}[H]
    \vspace*{-0.1in}
    \centering
    \begin{subfigure}{0.05\textwidth}
         \centering
         \includegraphics[width=\textwidth]{primaryfigs/compositionality_figs/hyper_activations/snowman/cluster-1.png}
     \end{subfigure}
     \begin{subfigure}{0.05\textwidth}
         \centering
         \includegraphics[width=\textwidth]{primaryfigs/compositionality_figs/hyper_activations/snowman/cluster-12.png}
     \end{subfigure}
     \begin{subfigure}{0.05\textwidth}
         \centering
         \includegraphics[width=\textwidth]{primaryfigs/compositionality_figs/hyper_activations/snowman/cluster-3.png}
     \end{subfigure}
     \begin{subfigure}{0.05\textwidth}
         \centering
         \includegraphics[width=\textwidth]{primaryfigs/compositionality_figs/hyper_activations/snowman/cluster-6.png}
     \end{subfigure}
     \begin{subfigure}{0.05\textwidth}
         \centering
         \includegraphics[width=\textwidth]{primaryfigs/compositionality_figs/hyper_activations/snowman/cluster-8.png}
     \end{subfigure}
    \caption{Sketches of snowmen with coloured cluster assignments.}
    \label{fig:snowman_hyper_activations_compose}
    \vspace*{-0.2in}
\end{figure}

\paragraph{Many classes: round objects}
We repeat the above experiment with a mixture of classes that generally can be expected to contain circles. These classes were circles, snowmen, clocks and cups. The two former classes are frequently composed only of circles, while the latter are expected to consistently contain other distinct shapes. Results are presented in Figure \ref{fig:allround_hyper_activations} and select examples in Figure \ref{fig:allround_hyper_activations_compose}.
\begin{figure*}[t]
    \vspace*{-0.1in}
    \centering
    \includegraphics[width=0.98\textwidth]{primaryfigs/compositionality_figs/hyper_activations/allround/collage.png}
    \caption{Clustering of hypernetwork activations of over many generated sketches of various classes of round objects. Left column is the full sketch, second are the ``noise'' strokes and every subsequent column is a unique cluster of stroke activations.}
    \label{fig:allround_hyper_activations}
    \vspace*{-0.2in}
\end{figure*} We still observe that the model continues to isolate circles in the first column and note it continues to do so for the cup and clock classes which are not exclusively circular.
\begin{figure}[H]
    \vspace*{-0.1in}
    \centering
    \begin{subfigure}{0.05\textwidth}
         \centering
         \includegraphics[width=\textwidth]{primaryfigs/compositionality_figs/hyper_activations/allround/cluster-1.png}
     \end{subfigure}
     \begin{subfigure}{0.05\textwidth}
         \centering
         \includegraphics[width=\textwidth]{primaryfigs/compositionality_figs/hyper_activations/allround/cluster-12.png}
     \end{subfigure}
     \begin{subfigure}{0.05\textwidth}
         \centering
         \includegraphics[width=\textwidth]{primaryfigs/compositionality_figs/hyper_activations/allround/cluster-13.png}
     \end{subfigure}
     \begin{subfigure}{0.05\textwidth}
         \centering
         \includegraphics[width=\textwidth]{primaryfigs/compositionality_figs/hyper_activations/allround/cluster-2.png}
     \end{subfigure}
     \begin{subfigure}{0.05\textwidth}
         \centering
         \includegraphics[width=\textwidth]{primaryfigs/compositionality_figs/hyper_activations/allround/cluster-9.png}
     \end{subfigure}
    \caption{Sketches of round objects with coloured cluster assignments.}
    \label{fig:allround_hyper_activations_compose}
    \vspace*{-0.2in}
\end{figure}

\paragraph{Many random classes:}
Finally, we repeat the above clustering with the 45 randomly selected holdout classes from the Quickdraw training process of \modelembedding{}. Results are once again presented in Figure \ref{fig:all_hyper_activations} and select examples in Figure \ref{fig:all_hyper_activations_compose}.
\begin{figure*}[t]
    \vspace*{-0.1in}
    \centering
    \includegraphics[width=0.98\textwidth]{primaryfigs/compositionality_figs/hyper_activations/all/collage.png}
    \caption{Clustering of hypernetwork activations of over many generated sketches of randomly selected classes. Left column is the full sketch, second are the ``noise'' strokes and every subsequent column is a unique cluster of stroke activations.}
    \label{fig:all_hyper_activations}
    \vspace*{-0.2in}
\end{figure*}
\begin{figure}[H]
    \vspace*{-0.1in}
    \centering
    \begin{subfigure}{0.05\textwidth}
         \centering
         \includegraphics[width=\textwidth]{primaryfigs/compositionality_figs/hyper_activations/all/cluster-0.png}
     \end{subfigure}
     \begin{subfigure}{0.05\textwidth}
         \centering
         \includegraphics[width=\textwidth]{primaryfigs/compositionality_figs/hyper_activations/all/cluster-1.png}
     \end{subfigure}
     \begin{subfigure}{0.05\textwidth}
         \centering
         \includegraphics[width=\textwidth]{primaryfigs/compositionality_figs/hyper_activations/all/cluster-15.png}
     \end{subfigure}
     \begin{subfigure}{0.05\textwidth}
         \centering
         \includegraphics[width=\textwidth]{primaryfigs/compositionality_figs/hyper_activations/all/cluster-5.png}
     \end{subfigure}
     \begin{subfigure}{0.05\textwidth}
         \centering
         \includegraphics[width=\textwidth]{primaryfigs/compositionality_figs/hyper_activations/all/cluster-7.png}
     \end{subfigure}
    \caption{Sketches of random classes with coloured cluster assignments.}
    \label{fig:all_hyper_activations_compose}
    \vspace*{-0.2in}
\end{figure}
