# Supplementary material for: SketchEmbedNet: Learning Novel Concepts by Imitating Drawings
Source: arXiv:2009.04806 source file (2021-06-22)
Supplement: Supplementary file 5 [file lin_readouts.tex]

\section{Latent Variable Recovery: Additional Results}
\label{appendix:lin_readouts}
We perform retrieval on the latent variable in the spatial relationships section with different amounts of data (100, 1000) as well as with a non-linear model. We also provide mean squared error as a metric.

\begin{table}[H]
\begin{minipage}[t]{0.48\textwidth}
    \begin{small}
        \begin{center}
            \caption{Spatial latent retrieval (1000)}
            \label{tab:alpha_values}
            \resizebox{0.98\textwidth}{!}{
            \begin{tabular}{@{}lcccc@{}}
                \toprule
                 & \multicolumn{2}{c}{\textbf{Linear}} & \multicolumn{2}{c}{\textbf{Non-Linear}} \\ \midrule
                 & $R^2$ & MSE & $R^2$ & MSE \\ \midrule
                Angle (\modelembedding{}) & 0.99 & 0.0013 & 0.98 & 0.0012 \\
                Angle (VAE) & 0.11 & 0.0793 & 0.95 & 0.0432 \\ \midrule 
                Distance (\modelembedding{}) & 0.97 & 0.090 & 0.98 & 0.058 \\ 
                Distance (VAE) & 0.28 & 2.287 & 0.97 & 0.092 \\ \midrule
                Size (\modelembedding{}) & 0.97 & 0.69 & 0.98 & 0.48 \\ 
                Size (VAE) & 0.20 & 21.72 & 0.98 & 0.44
            \end{tabular}}
        \end{center}
    \end{small}
\end{minipage}
\hfill
\begin{minipage}[t]{0.48\textwidth}
    \begin{small}
        \begin{center}
        \caption{Spatial latent retrieval (100)}
            \resizebox{0.98\textwidth}{!}{
            \begin{tabular}{@{}lcccc@{}}
                \toprule
                 & \multicolumn{2}{c}{\textbf{Linear}} & \multicolumn{2}{c}{\textbf{Non-Linear}} \\ \midrule
                 & $R^2$ & MSE & $R^2$ & MSE \\ \midrule
                Angle (\modelembedding{}) & 0.96 & 0.0037 & 0.95 & 0.0047 \\
                Angle (VAE) & 0.00 & 0.0969 & 0.82 & 0.0173 \\ \midrule 
                Distance (\modelembedding{}) & 0.82 & 0.585 & 0.96 & 0.14 \\ 
                Distance (VAE) & 0.00 & 3.24 & 0.91 & 0.28 \\ \midrule
                Size (\modelembedding{}) & 0.95 & 1.20 & 0.87 & 3.53 \\ 
                Size (VAE) & 0.02 & 26.70 & 0.85 & 4.01
            \end{tabular}}
        \end{center}
    \end{small}
\end{minipage}
\vspace{-0.15in}
\end{table}

We find that not only are \modelembedding{}s more effective with the same amount of data but also allow for identifying the latent spatial variable with far fewer examples.
