# Supplementary material for: SketchEmbedNet: Learning Novel Concepts by Imitating Drawings
Source: arXiv:2009.04806 source file (2021-06-22)
Supplement: Supplementary file 6 [file additional_concept_compt.tex]

\section{Additional Conceptual Compositionality}
\label{appendix:more_concept_comp}
\begin{figure*}
    \centering
    \includegraphics[trim=2cm 10cm 17.8cm 1.8cm,clip,width=0.88\textwidth]{primaryfigs/appendixfigs/more_cc_fig.pdf}
    \caption[]{Uncherrypicked conceptual compositionality examples}
    \label{fig:more_cc_examples}
\end{figure*}

\begin{figure*}
    \centering
    \includegraphics[trim=7cm 2.5cm 5.5cm 2.5cm,clip,width=0.99\textwidth]{primaryfigs/appendixfigs/concept_compo_additional.pdf}
    \caption[]{Additional conceptual compositionality examples}
    \label{fig:more_cc_setups}
\end{figure*}
