# Supplementary material for: SketchEmbedNet: Learning Novel Concepts by Imitating Drawings
Source: arXiv:2009.04806 source file (2021-06-22)
Supplement: Supplementary file 7 [file alpha_sweep.tex]

\section{Effect of $\alpha$ on Few-Shot Classification}
\label{appendix:alpha_sweep}

We performed additional experiments exploring the impact of our curriculum training schedule for $\alpha$. The encoding component of our drawing model was evaluated on the few-shot classification task for different values of $\alpha_\text{max}$ every 25k iterations during training. A graph is shown in Figure \ref{fig:alpha_time} and the full table of all values of $\alpha_\text{max}$ is in Table \ref{tab:alpha_time}.

\begin{figure}[H]
    \centering
    \includegraphics[width=0.48\textwidth]{primaryfigs/appendixfigs/alpha0and0p5.png}
    \caption{Few-shot classification accuracy of $\alpha_\text{max}$ values 0.0 and 0.5 over training}
    \label{fig:alpha_time}
\end{figure}

\begin{table*}
    \centering
    \caption{Few-shot classification accuracy of all $\alpha_\text{max}$ values}
    \resizebox{0.98\textwidth}{!}{
    \begin{tabular}{lllllllllllll}
        \toprule
        $\bm{\alpha_\text{max}}$ & \textbf{25k} & \textbf{50k} & \textbf{75k} & \textbf{100k} & \textbf{125k} & \textbf{150k} & \textbf{175k} & \textbf{200k} & \textbf{225k} & \textbf{250k} & \textbf{275k} & \textbf{300k}   \\
        \midrule
        0.00                & 89.35 & 87.94 & 88.73 & 88.46 & 88.01 & 88.04 & 88.23 & 87.73 & 88.03 & 87.86 & 87.65 & 87.17 \\
        0.25                & 89.21 & 90.39 & 90.20 & 89.75 & 87.78 & 88.37 & 88.64 & 88.05 & 87.98 & 88.41 & 88.15 & 87.82 \\
        0.50                & 90.48 & 89.58 & 89.81 & 89.02 & 90.68 & 91.24 & 90.26 & 90.94 & 91.12 & 91.30 & 91.12 & 91.39 \\
        0.75                & 91.39 & 89.95 & 89.56 & 89.81 & 89.95 & 90.79 & 91.02 & 91.09 & 91.82 & 90.76 & 91.42 & 90.59 \\ 
        0.95                & 90.23 & 90.15 & 90.10 & 89.55 & 90.27 & 92.37 & 92.27 & 90.29 & 91.58 & 91.02 & 89.73 & 89.77 \\
        \bottomrule
    \end{tabular}}
    \label{tab:alpha_time}
\end{table*}
