# Supplementary material for: SketchEmbedNet: Learning Novel Concepts by Imitating Drawings
Source: arXiv:2009.04806 source file (2021-06-22)
Supplement: Supplementary file 8 [file generation_discussion.tex]

\begin{figure*}[t]
    \centering
    \includegraphics[trim=0cm 0.22cm 0cm 0.2cm,clip,width=0.75\textwidth]{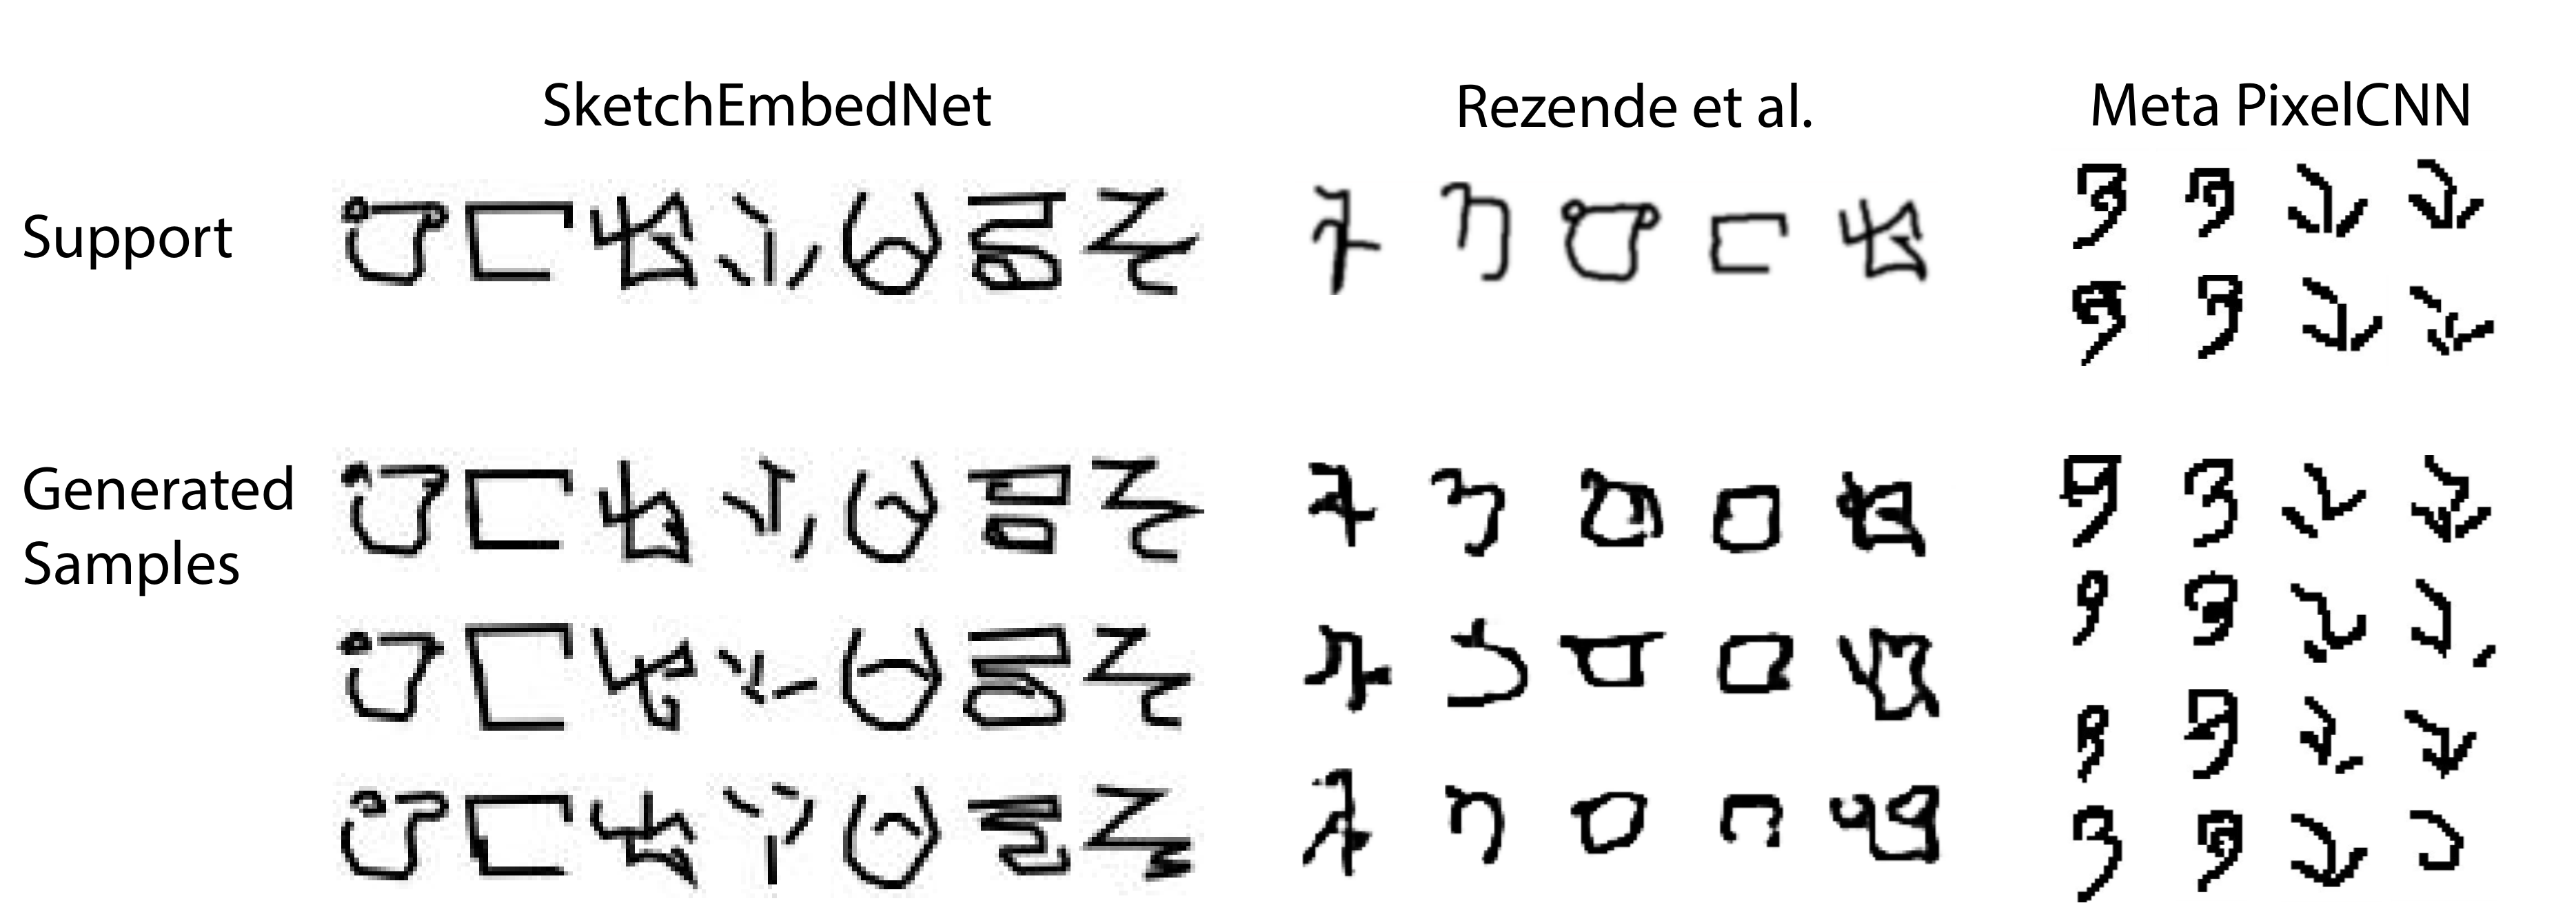}
    \caption{One-shot Omniglot generation compared to ~\citet{oneshotgen, fewshotgen}.}
    \label{fig:otherpapergenerations}
    \vspace{-0.15in}
\end{figure*}
\section{Generation cont.}
In addition to the Inception-score~\citep{inception} inspired metric, we also qualitatively assess the generative quality on unseen datasets. One-shot generations are sampled from the Omniglot~\citep{Lake2015bpl} and are qualitatively compared to other one-shot and few-shot generation methods~\citep{oneshotgen, fewshotgen} (Figure \ref{fig:otherpapergenerations}. 

None of the models have seen any examples from the character class or parent alphabet. Furthermore \model{} has not encountered any Omniglot examples during training. Visually, our generated images better resemble the support examples and the variations by stretching and shifting strokes better preserves the semantics of each character. Generations in pixel space may disrupt strokes and alter the character to human perception. This is especially true for written characters as they are frequently defined by a specific set of strokes instead of blurry clusters of pixels.
