# Supplementary material for: SketchEmbedNet: Learning Novel Concepts by Imitating Drawings
Source: arXiv:2009.04806 source file (2021-06-22)
Supplement: Supplementary file 9 [file intra_class_discussion.tex]

\section{Embedding informativeness and Generation Quality}
While it is intuitive that a well-trained generative model should present an informative embedding and vice-versa, performing well on a generative task may not be sufficient to produce a useful embedding. Section 4.3 and 4.5 both perform classification on unseen examples of the Omniglot training dataset, the former on latent representations and the latter on decoded images. While absolute accuracy is not meaningful due to classifier and task differences, the Conv-VAE~\citep{vae} performs substantially better on the generation classification task compared to its performance in embedding classification. 

We believe this highlights an important difference between generative models that operate in pixel space compared to other decoding representations. We believe it is because of the unique and structured properties of sequential sketching (discussed in Section 4.4) that motivate a more specific understanding of the components and relationships in the image that enable our \modelembedding{}s superior informativeness.
