# Supplementary material for: SketchEmbedNet: Learning Novel Concepts by Imitating Drawings
Source: arXiv:2009.04806 source file (2021-06-22)
Supplement: Supplementary file 10 [file intro.tex]

\begin{abstract}
    In our supplementary materials we provide implentation details, additional experimental results and further exploration of our latent embeddings. We also present our results for the lesser addressed Lake split \citep{Lake2015bpl} of the Omniglot few-shot classification benchmark, detail on our differentiable rasterization function $f_\text{raster}$ and our data processing procedures.
\end{abstract}
