# Supplementary material for: SketchEmbedNet: Learning Novel Concepts by Imitating Drawings
Source: arXiv:2009.04806 source file (2021-06-22)
Supplement: Supplementary file 11 [file additional_experiments.tex]

\section{Additional Experiments}
%Was going to explore the over train time and over pixel_weight sweep here. Definitely won't fit now.
